# Supplementary material for: Couplings of the Random-Walk Metropolis algorithm
Source: arXiv:2102.01790 source file (2021-02-02)
Supplement: Supplementary file 1 [file appendix.tex]

% !TEX root = text.tex

%%%%%%%%%%%%%%%%%%

\section{Notes and todos}

%%%
\subsection{Section \ref{sec:couplings:defn}}

\begin{itemize}

\item The Wang paper on full kernel couplings doesn't exist yet. We should add that when possible. We could also sketch such couplings here or talk about their properties (slightly higher chance of meeting, harder to work with because lack of nice symmetries). I am inclined not to do, since there's so much here already and we are working with Guanyang on it.

\item If desired, we could state and prove a lemma saying that if we start with any coupling of initial conditions, proposals, and accept/reject steps, then we can find a corresponding sticky/faithful coupling by switching to the same proposal and accept/reject once the chains meet.

\item This observation is consistent with Proposition 3 of \citet{Dey2017}, which shows that the convertibility of a general Markovian coupling into a sticky one is equivalent to a condition similar to the strong Markov property holding for both chains with respect to the stopping time $\tau$.

\item Here or in the section on initialization, we should mention that the time convention here is different from the Unbiased MCMC paper in that here we are looking for $X_t = Y_t$. When it's important for $X_1 \sim Y_0$, we will describe it as $X_{-L}, Y_0 \sim \pi_0$ for some lag $L$.

\item For now, we consider a hybrid method which employs the reflection-maximal coupling only on a set $\calC$ where the chains are likely to meet. See Section \ref{max_coupling} for details. Otherwise we use the simple reflection coupling, in which we draw $\xi \sim \N(0, I_d \, \ell^2 / d)$ and set $\eta = (I_d - 2 ee') \xi$. The reflection and reflection-maximal coupling are related by Lemma \ref{reflection_max}, below, which implies that they coincide with high probability except for small $r$.

\item Let ${\delta = ||y||^2 - ||x||^2}, \Delta = ||Y||^2 - ||X||^2, m = (x+y)/2$, and ${M=(X+Y)/2}$.
Note that $\delta = y_1^2 - x_1^2$, $m_1 = e'm = \delta / (2r)$, and $M_1 = \Delta / (2R)$.
For any events $A, B,$ and random variable $Z$,
we write $A \symdiff B := (A \cap B^c) \cup (A^c \cap B)$
and $\E[Z ; A ] := \E[Z\, 1(A)]$.

\end{itemize}

%%%
\subsection{Section \ref{sec:couplings:props}}
\begin{itemize}

\item We could mention the expected computational cost of the maximal coupling, and the variant that delivers slightly less than a maximal coupling but with a more controlled variance.

\item Pollard [2005] is a set of lecture notes here: \url{http://www.stat.yale.edu/~pollard/Courses/607.spring05/handouts/Totalvar.pdf}. This is better than a mathoverflow page, but I wonder if there is a more official published reference for this result?

\item Should we give the algorithm for drawing from the maximal coupling with independent residuals?

\item Maybe we should also describe the radial coupling? Here or in an appendix? It involves a lot of fun stuff about spherical distributions.

\item Also maybe the `full' reflection coupling where we also reflect $\xn$. This never performs that well, so it seems unnecessary to clutter things further with a coupling that is worse than the max independent version.

\end{itemize}

%%%
\subsection{Section \ref{sec:mt_sims}}
\begin{itemize}

\item We could include simulations on accept/reject couplings here, although it's unclear if we should.

\end{itemize}

%%%
\subsection{Bibliography}
\begin{itemize}

\item Most of these bibliography items are automatically generated from Google scholar or Mendeley, and as such are not way off but include typos and odd formatting issues. Very important to proofread these.

\end{itemize}

\pagebreak
